# Supplementary material for: Strong Momentum-Dependent Electron-Magnon Renormalization of a Surface Resonance on Iron
Source: arXiv:2108.03421 source file (2021-08-07)
Supplement: Supplementary file 1 [file SM_FePaper_v4.0.pdf]

# Supplemental Material

## Strong Momentum-Dependent Electron-Magnon Renormalization of a Surface Resonance on Iron

Beatrice Andres and Martin Weinelt\*

*Freie Universität Berlin, Fachbereich Physik, Arnimallee 14, 14195 Berlin, Germany*

Hubert Ebert and Jürgen Braun

*Ludwig-Maximilians-Universität München, Butenandtstr. 5-13, 81377 München, Germany*

Alex Aperis and Peter M. Oppeneer

*Department of Physics and Astronomy, Uppsala University, P. O. Box 516, 75120 Uppsala, Sweden*

(Dated: July 27, 2020)

### SETUP FOR SPIN-POLARIZED PHOTOEMISSION

The photoemission experiments were performed with the exchange-scattering spin-detector described in [1] in combination with a cylindrical sector analyzer. The incoming electron beam is backscattered at an incidence angle of  $15^\circ$ . As a scattering target, the spin detector uses an oxygen-passivated 6 ML-thick Fe/W(001) film. Spin-resolution is achieved by reversing the magnetization of the Fe target. Thus, it is possible to perform spin-resolved measurements while keeping the sample magnetization and the measurement geometry unchanged. This ensures that the observed magnetic linear dichroism (Fig. 2, main text) is not compromised by the spin polarization and vice versa. The angle-resolved spectra were measured along the  $\bar{\Gamma} - \bar{H}$  direction ( $\equiv [001]$ ). The angular resolution was  $\pm 2.5^\circ$ .

All direct photoemission data presented in the main text and supplement were measured on the same sample. As a photon source, we used the fourth harmonic (6.3 eV) of an amplified Ti:Sapphire laser. A second and third sample was measured in direct photoemission to confirm the results of this work. (The data is available from the corresponding author on reasonable request.)

### SAMPLE PREPARATION

The 15-ML-thick Fe(110) samples were grown *in situ* on a W(110) substrate, that was cleaned beforehand by oxygen treatment. Fe was evaporated from a 2-mm rod (purity 99.995 %) in an EFM3 evaporator (Focus, Omicron). The deposition rate was 2 Å per minute. The first 2 ML were grown at 300 K. During deposition of the subsequent layers, the temperature was raised to 530 K at a rate of 1.5 K/s, where it was kept during the remaining evaporation and for 10 minutes additional annealing time. The easy magnetization axis for the 15-ML-thick Fe film lies along the  $[1\bar{1}0]$  direction [2]. The sample was magnetized by field pulses through an air-wound coil.

### ELECTRONIC STRUCTURE AND SPECTROSCOPICAL ANALYSIS

The self-consistent electronic structure calculations were performed within the *ab initio* framework of spin-density functional theory, in a fully relativistic mode by solving the corresponding Dirac equation. For the exchange and correlation potential the Perdew-Burke-Ernzerhof parameterization was used [3]. To account for electronic correlations beyond the local spin-density approximation (LSDA) we employed a self-consistent combination of the LSDA and the dynamical mean field theory. This computational LSDA+DMFT scheme, self-consistent in both the self-energy calculation and the charge-density calculation is implemented within the relativistic SPR-KKR formalism [4]. In the present study we used for the on-site Coulomb interaction a value  $U = 1.5$  eV, and for the averaged on-site exchange interaction a value  $J = 0.9$  eV [5].

The spectroscopical analysis is based on the fully relativistic one-step model in its spin-density matrix formulation [6]. The final state is constructed within spin-polarized low-energy electron diffraction (SPLEED) [7]. In addition for the photoemission calculations, the solid surface is accounted by a Rundgren-Malmström-type potential [8]. As this surface barrier represents a  $z$ -dependent potential, a surface contribution as part of the total photocurrent results, which accounts explicitly for the energetics and dispersion of all surface features. Furthermore, the relative intensities of surface-related spectral features are quantitatively accounted for by calculating the corresponding matrix elements in the surface region. This procedure is described in detail, for example, in [9]. For the photoemission calculations we used a spin-dependent Rundgren-Malmström barrier in the parametrization which has been successfully applied in a previous study on Fe(110) [10]. Life-time effects in the initial states have been accounted for via the imaginary part  $\text{Im}\Sigma^{DMFT}$  of the energy-dependent DMFT-type self-energy. To take care of impurity scattering, a small constant imaginary value of  $V_{i1} = 0.005$  eV has

been added to  $\text{Im}\Sigma^{DMFT}$ . Life-time effects in the final state are accounted for by the imaginary part of the inner potential. A constant imaginary value of  $V_{i2} = 1.5 \text{ eV}$  has been chosen in a phenomenological way. Due to the finite imaginary part, the inelastic mean free path (IMFP) is accounted for. In this way the amplitude of the photoelectron state can be neglected beyond a certain distance from the surface. According to the experimental setup the spectroscopic calculations were performed for linearly  $p$ -polarized light and a photon energy of  $6.3 \text{ eV}$ .

### MINORITY-SPIN CHARACTER OF THE SURFACE RESONANCE

Our one-step photoemission calculations corroborate the strong *minority-spin* character of the surface resonance. Fig. S1 depicts the spin polarization in the range of the surface resonance along  $\bar{\Gamma} - \bar{\text{H}}$ . The  $E$  vs.  $k_{\parallel}$  range is the same as in Fig. 1(b) of the main text. The calculation reflects the main peak seen in photoemission and its minority spin character. The large exchange splitting in Fe shifts the corresponding *majority-spin* surface resonance above the Fermi level  $E_F$ . Alongside strong spin-orbit coupling, there are points  $E(\mathbf{k})$  in the band structure at which majority- and minority-spin bands hybridize differently. This also creates independent conditions for majority- and minority-spin surface states to form. As a consequence, the majority-spin part of the surface resonance is shifted above  $E_F$  and is dispersing upward, while below  $E_F$  the minority-spin component disperses downward for off-normal emission [10].

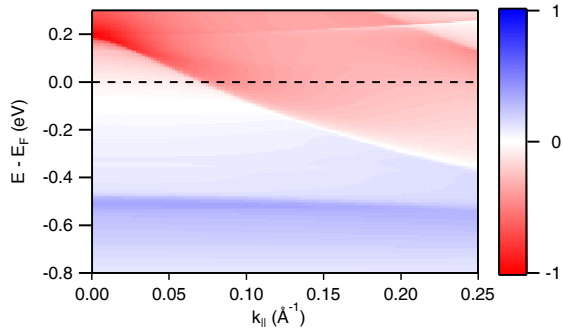

FIG. S1. One-step photoemission calculation of the spin polarization of the surface resonance based on the LSDA+DMFT electronic structure calculation. The calculation uses the experimental photon energy of  $6.3 \text{ eV}$  and confirms the minority spin character (red) of the surface resonance (main peak in photoemission).

### SPATIAL CHARACTER OF THE MINORITY SURFACE RESONANCE

In the main text we discussed the  $\Sigma_{3,1}$  spatial symmetry character of the surface resonance. We confirmed this assignment in an additional two-photon photoemission (2PPE) experiment on a fourth sample which we describe below.

In our 2PPE experiment pump and probe laser pulses are used to excite electrons from an occupied initial state below the Fermi energy  $E_F$  via an unoccupied intermediate state below the vacuum level  $E_{vac}$  into the continuum. With the third harmonic of a Ti:Sapphire oscillator as pump pulse ( $3h\nu = 4.83 \text{ eV}$  photon energy), we can thereby project the occupied part of the band structure (initial state) onto the total symmetric  $n = 1$  image-potential state of Fe(110). This intermediate state is ionized by the laser fundamental, which serves as probe pulse ( $h\nu = 1.61 \text{ eV}$ ). The approach has been used to study the exchange splitting of image-potential states [11, 12].

In the experiment, both beams were incident at an angle of  $80^\circ$  along the  $[001]$  direction and the sample was rotated around the polar angle  $\vartheta$  to record angle-resolved 2PPE spectra (*cf.* Fig. S2). The spin- and angle-resolved 2PPE data are summarized in Figs. S3(a) and (b). Transitions between initial bulk states and the bottom of the  $n = 1$  image-potential-state band ( $\vartheta = 0^\circ$ ) are depicted in the left panel of Fig. S3(c) by vertical arrows.  $\Gamma\text{N}$  corresponds to the direction along the Fe(110) surface normal. Transitions between the surface resonance (red dots) and the  $n = 1$  image-potential-state band are depicted in the surface-projected bulk band-structure along  $\bar{\Gamma} - \bar{\text{H}}$  (right panel of Fig. S3(c)).

As sketched in Fig. S2, for normal emission and  $p$ -polarized light the vector potential  $\mathbf{A}$  is nearly perpen-

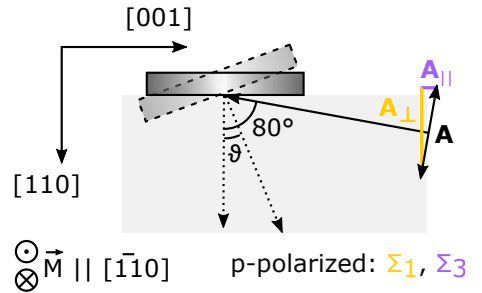

FIG. S2. Experimental geometry of the two-photon photoemission measurement. For grazing incidence at an angle of  $80^\circ$  along the  $[001]$  azimuth the vector potential is nearly perpendicular to the surface  $\mathbf{A} \sim \mathbf{A}_\perp$ . Therefore dipole transitions between initial states of  $\Sigma_1$  symmetry and the total symmetric  $n = 1$  image-potential state dominate. For larger emission angles  $\vartheta$  the parallel component of the vector potential  $\mathbf{A}_\parallel$  and thus the transition probability from  $\Sigma_3$  initial states increases.

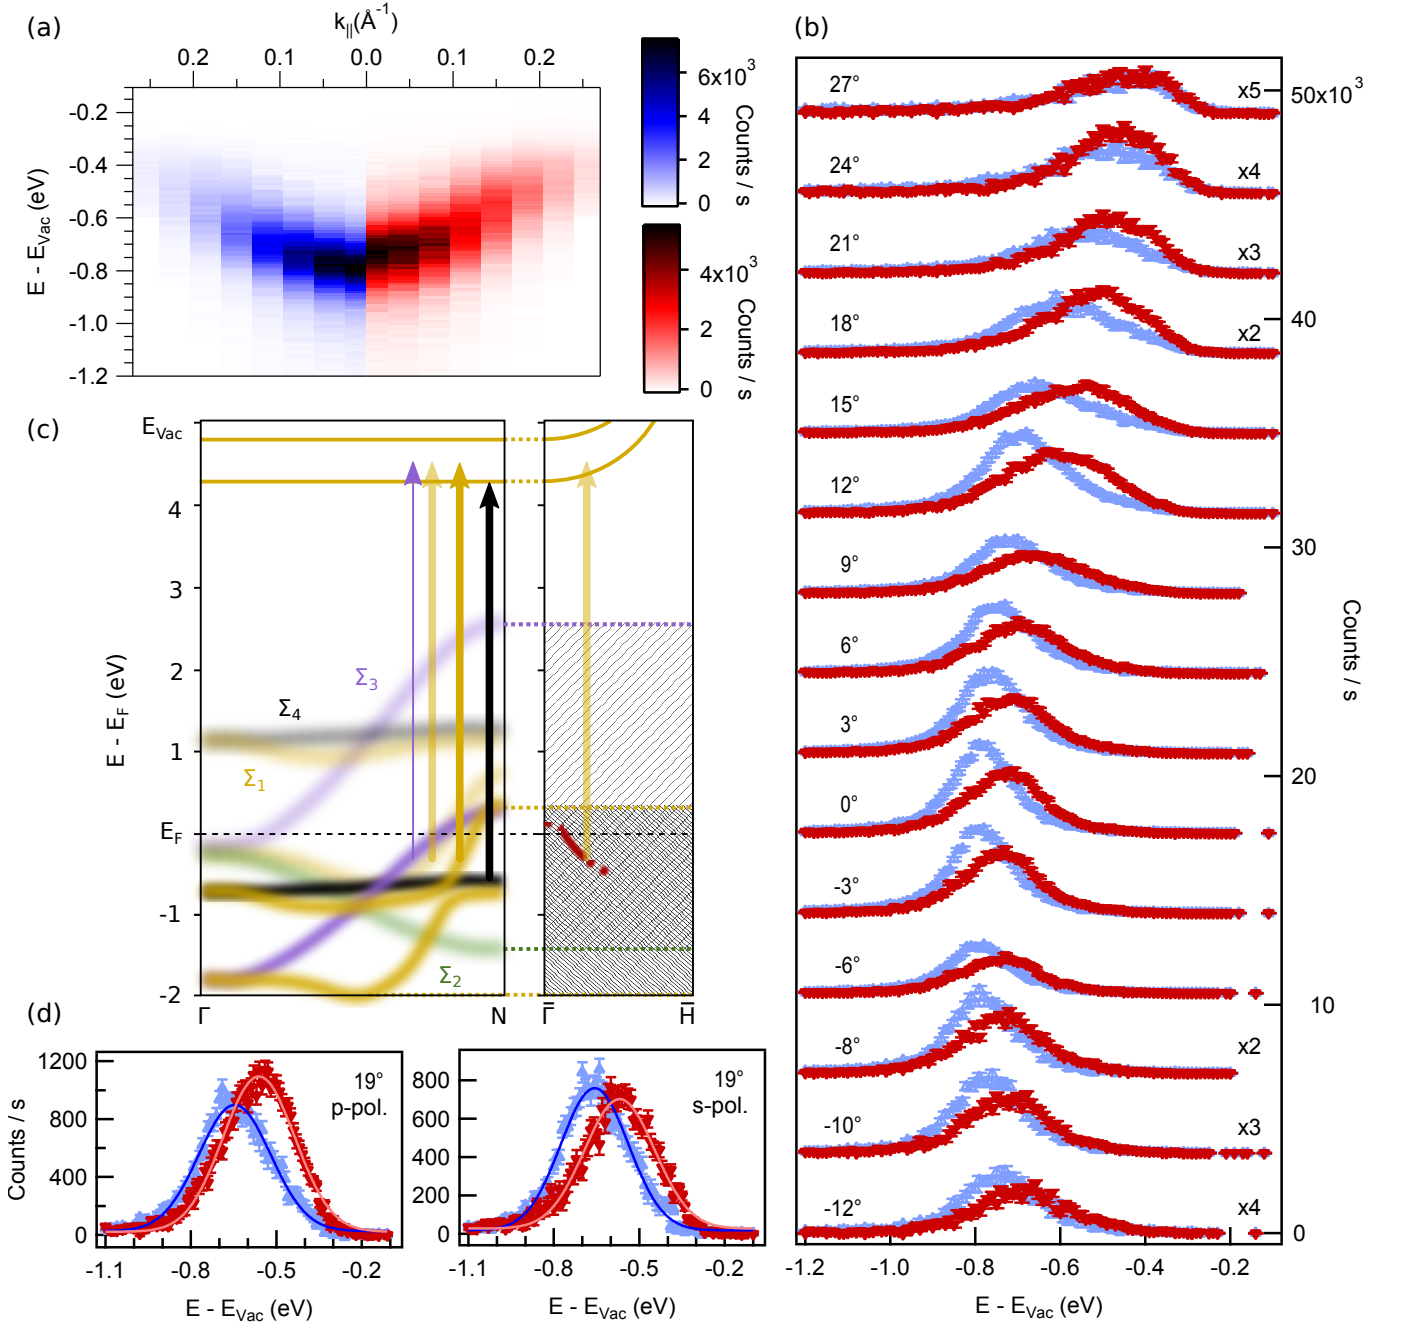

FIG. S3. (a) and (b) Majority- (blue) and minority-spin (red) 2PPE intensities from the  $n = 1$  image-potential state upon excitation with  $p$ -polarized light. (c) Schematic explanation of the different pathways of photoexcitation from the surface and surface-projected bulk band-structure into the image-potential states (band structure redrawn from Ref. [5]). Majority-spin bands are drawn opaque, minority-spin bands half-transparent. The left side shows the bulk band structure along the  $\Gamma - N$  direction perpendicular to the crystal surface. The right side shows this band structure projected onto the center of the surface Brillouin zone  $\bar{\Gamma}$  (majority- and minority-spin band structure shaded differently) together with the dispersion of surface states along  $\bar{\Gamma} - \bar{H}$ . (d) Changing the spin character by excitation using  $p$ - and  $s$ -polarized pump pulses.

pendicular to the crystal surface. The  $\mathbf{A}_{\perp}$  component excites electrons from  $\Sigma_1$  initial states into the  $n = 1$  image-potential state of  $\Sigma_1$  character (yellow arrows in Fig. S3(c)). With increasing emission angle  $\vartheta$ , the increasing  $\mathbf{A}_{\parallel}$ -component allows for additional excitation from

$\Sigma_3$  states (purple arrow).

The real part of the wave vector of the  $n = 1$  image-potential state in the bulk corresponds to the  $k$ -vector at the Brillouin zone boundary  $\text{Re}(k_{\perp}) = k_N$ . Based on the spatial overlap with the  $n = 1$  image-potential

state, initial bulk states near the N point will contribute predominantly to the transition matrix-element of the pump step. We measured a work function of  $\Phi = 5.0$  eV for the Fe(110) films. The binding energy of the  $n = 1$  image-potential state with respect to the vacuum level is 0.77 eV. Thus with a pump pulse photon energy of 4.83 eV we can probe initial bulk states up to 0.6 eV below the Fermi level  $E_F$  near the N point.

At the bottom of the parabolic dispersion of the image-potential state, we find the projection of a band with majority-spin character (Fig. S3 (b),  $\vartheta = 0^\circ$ ). Since there are no occupied surface states of majority-spin character in the available energy range, the transition is assigned to the majority spin  $\Sigma_1$  bulk band that crosses  $E_F$  near the N point (highlighted opaque yellow in Fig. S3 (c)).

Rotating the sample to off-normal emission we find a change of the  $n = 1$  spin-polarization to minority-spin character. Furthermore, the dispersion of the minority-spin branch starts to deviate from the parabolic shape which can still be observed for the majority-spin branch. Since all data were recorded for overlapping pump and probe pulses ( $\Delta t = 0$ ), the change in spin-polarization and dispersion is attributed to an initial state effect. As described in the main text, we find the minority-spin surface resonance at the Fermi level dispersing downwards to become occupied at about  $0.08 \text{ \AA}^{-1}$  (indicated by red dots in the right panel of Fig. S3 (c)). Since the wave function of the surface resonance has a higher overlap with the image-potential-state wave function as compared to bulk states, it will dominate the 2PPE spectra. This starts for parallel momenta where the minority-spin surface resonance becomes occupied.

At small emission angles, we exclusively observe the projection of the  $\Sigma_1$  and  $\Sigma_3$  bulk bands of mixed majority- and minority-spin character onto the image-potential state. For parallel momenta above  $0.08 \text{ \AA}^{-1}$ , which correspond to  $\vartheta \geq 10^\circ$ , transitions from the minority-spin surface resonance (red dashed line in Fig. S3(c), right panel) add minority spin-character and change the dispersion of the minority-spin component of the  $n = 1$  image-potential state.

To corroborate that the minority-spin character in the image-potential state stems from the  $\Sigma_{1,3}$  surface resonance at  $E_F$ , we changed the initial state by switching the pump-light polarization from  $p$  to  $s$ . This changes the initial state symmetry-character from  $\Sigma_{3,1}$  to  $\Sigma_4$  (black arrow in Fig. S3 (c)). As expected, the 2PPE spectra in Fig. S3 (d) show a reduction of the minority-spin character, when switching the light polarization from  $p$  to  $s$ . With  $s$ -polarized light, dipole transitions from the  $\Sigma_{3,1}$  surface resonance into the  $\Sigma_1$  image-potential state are forbidden.

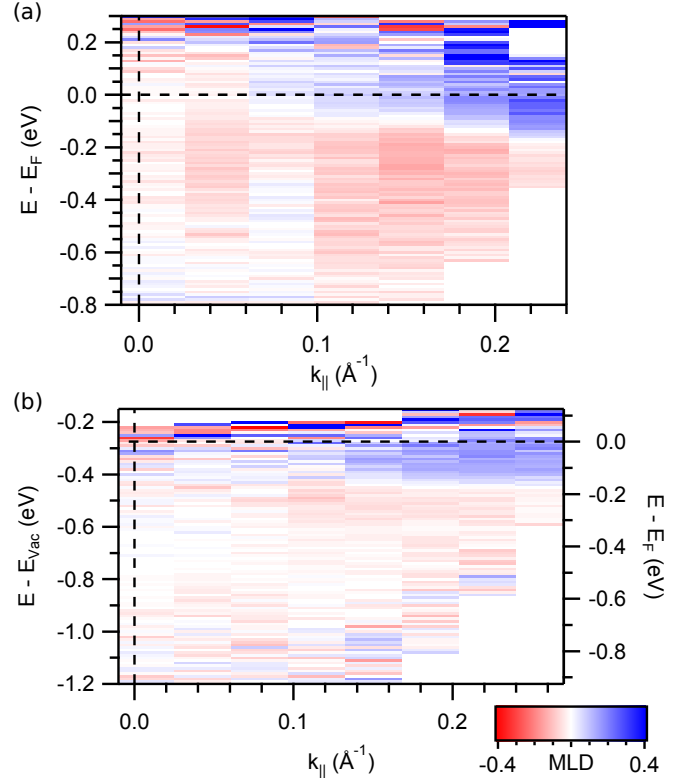

FIG. S4. (a)  $E(k_{\parallel})$  map of the magnetic linear dichroism extracted from all minority-spin spectra shown in Fig. 1(a) of the main text and the minority-spin spectra recorded for opposite magnetization direction as exemplary shown in Fig. 2 of the main text. We find an increase of intensity in the resonance close to  $E_F$  (right ordinate) and a decrease of intensity in the resonance for  $E - E_F \geq 160$  meV. (b) Magnetic linear dichroism extracted from the two-photon photoemission spectra shown in Fig. S3 (b) and spectra recorded for reversed magnetization (not shown). The overall MLD contrast is comparable to direct photoemission and corroborates the decrease of intensity in the surface resonance for  $E - E_F \geq 160$  meV.

## MAGNETIC LINEAR DICHROISM

Figure 2 of the main text shows pairs of minority-spin spectra with the sample magnetized in opposite directions, *i.e.*, for spin magnetic moments aligned antiparallel to M+ and M-, respectively. A complete  $E(k_{\parallel})$  map of the magnetic linear dichroism (MLD) is shown in Fig. S4 (a). Reversing the direction of the sample magnetization, we find an increase of the photoemission intensities close to  $E_F$  and a loss of intensity, when the binding energy exceeds a value of 160 meV. The binding energy at which the dichroism changes its sign must be the energy of the excited and reabsorbed magnons. From Fig. S4 we extract a value for the magnon energies of  $\approx 160$  meV, which is compatible with the optical magnon branch (see Fig. S5).

We likewise find MLD in our 2PPE measurements depicted in Fig. S4. The left ordinate refers to the binding-

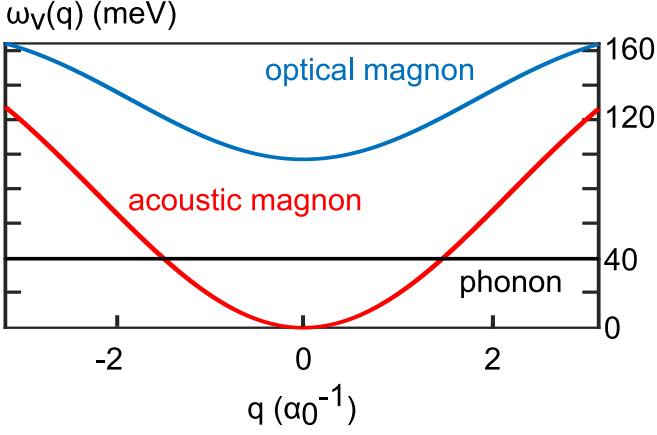

FIG. S5. Dispersions  $\omega_\nu(\mathbf{q})$  of the acoustic and gapped optical magnon modes and of the considered Einstein phonon mode.

energy scale of the  $n = 1$  image-potential state, the right ordinate scale to the initial state energy scale. MLD again develops for finite parallel momenta ( $k_{\parallel}$  above  $0.08 \text{ \AA}^{-1}$ ), where the surface resonance is occupied.

The occurrence of the MLD in 2PPE as well as direct photoemission further corroborates the hypothesis of electron-magnon renormalization causing the observed effects. If the magnons couple stronger to the electrons for one magnetization direction, this should lead to a shift of intensities from the bare to the renormalized peak. Such a shift must be observable as MLD both in direct and two-photon photoemission. The occurrence of magnetic linear dichroism implies that the electron-magnon renormalization depends on the crystal momentum of the interacting electrons and magnons.

## QUASIPARTICLE SPECTRUM CALCULATIONS

Electron-boson interaction leads to a quasiparticle renormalization of the bare electronic band. As outlined in the main text, we consider three different boson modes, an acoustic magnon, a gapped optical magnon and a dispersionless Einstein phonon mode with frequency  $\Omega_0 = 40 \text{ meV}$ . The dispersions of these boson modes are shown in Fig. S5. For the acoustic and optical magnon modes we used the parametrization in terms of Heisenberg constants as given in Ref. [13] (see main text), which is consistent with *ab initio* calculations for the bulk magnon mode of bcc iron [14].

For these bosonic modes we compute the spectral function which is proportional to the photoemission spectrum while varying the interaction strength  $I_\nu$  (for mode  $\nu$ ). The calculated spectral functions are given in Fig. S6.

From Fig. S6(a) it can be observed that interaction with the phonon mode leads to a renormalized electron dispersion that exhibits a change of slope that is commonly referred to as a phonon-induced kink. The arrows

indicate the positions of the phonon kinks that originate from the phonon propagator. One of these appears close to the Fermi energy  $E_F$  because of the involved small phonon frequency, and a second kink appears at higher binding energy than the bare band dispersion. Evidently, the quasiparticle band shown in Fig. S6(a) does not display any replica features, i.e., a single dispersive band at about 200 meV binding energy is found, in clear contrast to the ARPES measurements shown in Fig. 1(a). The situation is markedly different in the case of electrons coupling to the acoustic magnon mode, as shown in Fig. S6(b). The resulting interaction in this case is strongly peaked for small wavevector exchange, thus producing a replica band which manifests itself in the spectra as a split-off quasiparticle peak. However, this splitting requires unrealistically large coupling constants ( $\lambda \gg 3.6$ ) to produce a sizable effect. In addition, the peak that is closer to the Fermi level always has the biggest height, in contrast to what is observed experimentally (see Fig. 1(a)). In Fig. S6(c) we plot the results obtained for the gapped optical magnon; these are the same spectra as shown in Fig. 3 of the main text. Evidently, the resulting spectra due to coupling of the electrons to the optical magnon mode not only exhibit the observed split-off peak, i.e., the replica-band formation, at the correct energies, but in addition, the heights of the calculated peaks are in good qualitative agreement with experiment as well. Consequently, the observed momentum-dependent replica-band formation of the surface resonance is consistently explained by strong electron-magnon interaction to a gapped optical magnon mode.

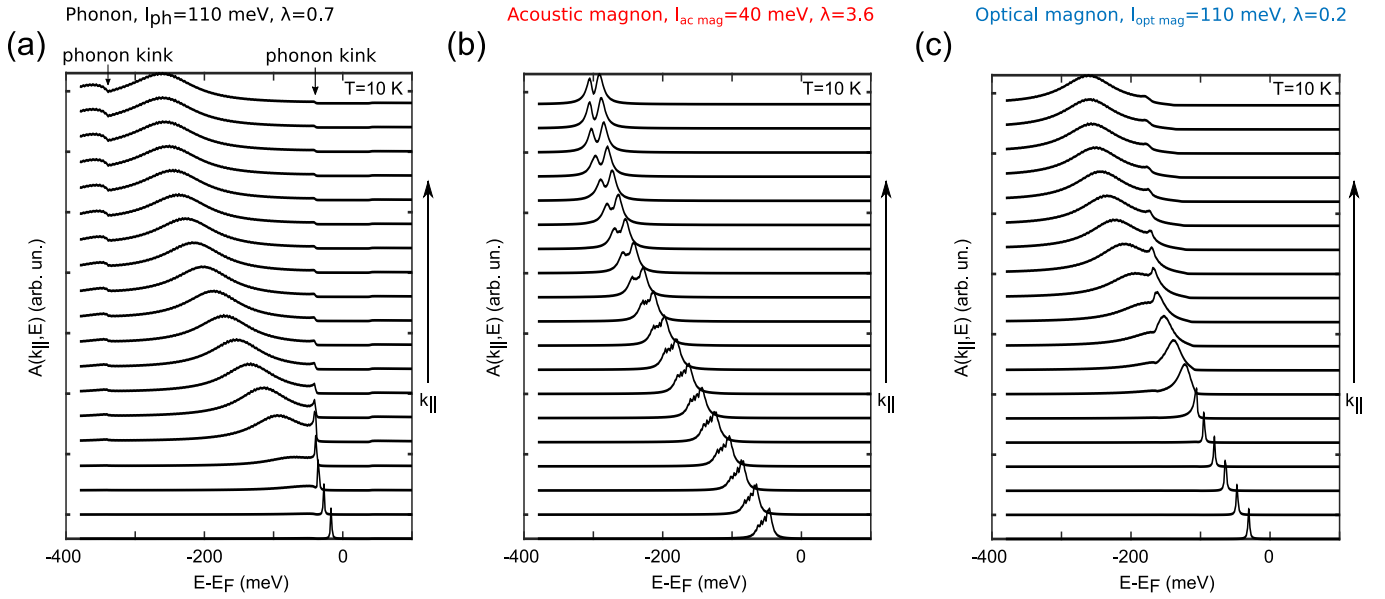

FIG. S6. Calculated spectral function of the renormalized surface state, assuming electron-boson coupling of the electrons to (a) an Einstein phonon, (b) an acoustic magnon, and (c) an optical magnon mode. The strength of the electron-boson interaction  $I$  and the computed corresponding electron-boson coupling constant  $\lambda$  for each case are displayed above each panel.

\* Corresponding author: weinelt@physik.fu-berlin.de

- [1] A. Winkelmann, D. Hartung, H. Engelhard, C.-T. Chiang, and J. Kirschner, *Rev. Sci. Instrum.* **79**, 083303 (2008).
- [2] M. Slezak, T. Giela, D. Wilgocka-Slezak, A. Koziol-Rachwal, T. Slezak, R. Zdyb, N. Spiridis, C. Quitmann, J. Raabe, N. Pilet, and J. Korecki, *J. Magn. Magn. Mater.* **348**, 101 (2013).
- [3] J. P. Perdew, K. Burke, and M. Ernzerhof, *Phys. Rev. Lett.* **77**, 3865 (1996).
- [4] J. Minár, J. Braun, and H. Ebert, *J. Elect. Spec. Rel. Phenom.* **189**, 129 (2013).
- [5] J. Sánchez-Barriga, J. Fink, V. Boni, I. Di Marco, J. Braun, J. Minár, A. Varykhalov, O. Rader, V. Bellini, F. Manghi, H. Ebert, M. I. Katsnelson, A. I. Lichtenstein, O. Eriksson, W. Eberhardt, and H. A. Dürr, *Phys. Rev. Lett.* **103**, 267203 (2009).
- [6] J. Braun, K. Miyamoto, T. Okuda, M. Donath, A. Kimura, H. Ebert, and J. Minár, *New J. Phys.* **16**, 015005 (2014).
- [7] J. Braun, J. Minár, and H. Ebert, *Phys. Rep.* **740**, 1 (2018).
- [8] G. Malmström and J. Rundgren, *Phys. Commun.* **19**, 263 (1980).
- [9] A. Nuber, J. Braun, F. Forster, J. Minár, F. Reinert, and H. Ebert, *Phys. Rev. B* **83**, 165401 (2011).
- [10] J. Braun, C. Math, A. Postnikov, and M. Donath, *Phys. Rev. B* **65**, 184412 (2002).
- [11] W. Wallauer and T. Fauster, *Phys. Rev. B* **54**, 5086 (1996).
- [12] M. Pickel, A. B. Schmidt, M. Weinelt, and M. Donath, *Phys. Rev. Lett.* **104**, 237204 (2010).
- [13] Y. Zhang, *High wave vector spin waves in ultrathin Fe films on W(110) studied by spin-polarized electron energy loss spectroscopy*, Ph.D. thesis, Martin-Luther University, Halle-Wittenberg, Germany (2009).
- [14] S. V. Halilov, H. Eschrig, A. Y. Perlov, and P. M. Oppeneer, *Phys. Rev. B* **58**, 293 (1998).
